# Supplementary material for: Enhancing Noise-Robust Losses for Large-Scale Noisy Data Learning
Source: arXiv:2306.05497 source file (2025-01-27)
Supplement: Supplementary file 1 [file Supplement.pdf]

---

# Supplemental Material — Reevaluating Loss Functions: Enhancing Robustness to Label Noise in Deep Learning Models

---

**Max Staats \***

Institut für Theoretische Physik  
Universität Leipzig  
Brüderstraße 16, 04103 Leipzig  
staats@itp.uni-leipzig.de

**Matthias Thamm**

Institut für Theoretische Physik  
Universität Leipzig  
Brüderstraße 16, 04103 Leipzig  
thamm@itp.uni-leipzig.de

**Bernd Rosenow**

Institut für Theoretische Physik  
Universität Leipzig  
Brüderstraße 16, 04103 Leipzig  
rosenow@physik.uni-leipzig.de

## 1 Details on preprocessing

When training ResNet networks, we normalize Cifar-10 images by subtracting the mean  $\mu = (0.485, 0.456, 0.406)$  and then dividing by  $\sigma = (0.229, 0.224, 0.225)$  for the three color channels. On each training data batch, we further perform a random horizontal flip followed by random cropping to size  $32 \times 32$  with a padding of size 4.

For training ResNet on Fashion-MNIST, we normalize the black and white images using  $\mu = 0.286$  and  $\sigma = 0.353$ . Batches during training are processed with a random horizontal flip followed by random cropping to a size  $28 \times 28$  with a padding of size 4.

The Cifar-100 dataset is normalized using  $\mu = (0.507, 0.487, 0.441)$  and  $\sigma = (0.267, 0.256, 0.276)$  and the training data is processed with random cropping ( $32 \times 32$ , padding 4), followed by a random horizontal flip, and a random rotation by up to  $15^\circ$ .

For training MLP1024 networks, we only normalize the images. All test data is normalized identically to the corresponding training data and no further processing is performed.

## 2 Learning rate optimization for MLP1024 networks

For training MLP1024 networks on the Cifar-10 and Fashion-MNIST dataset, we perform a grid search over nine values of initial learning rates in the absence of label noise. The value with the best average accuracy out of five runs for each learning rate is then used for training in the presence of varying degrees of label noise. This allows a more balanced comparison of the different loss functions in the case of the MLP1024 networks, where we observe a stronger dependence on the initial learning rates than in the case of ResNet (results for the learning rate dependence of ResNet not shown). The results for MLP1024 networks are shown in Table 1 where values in a bold font mark the learning rate used in the main text.

---

\*Corresponding author.

Table 1: Learning rate optimization for various loss functions on the clean dataset for MLP1024 networks. The test accuracies in bold face indicates the learning rate for which results are presented in the main manuscript. MAE\* has  $\epsilon = 0.5$

| learning rate | 0.0005           | 0.0008                  | 0.001                   | 0.003                   | 0.005                   | 0.008            | 0.01                    | 0.03             | 0.05             |
|---------------|------------------|-------------------------|-------------------------|-------------------------|-------------------------|------------------|-------------------------|------------------|------------------|
| Cifar-10      |                  |                         |                         |                         |                         |                  |                         |                  |                  |
| CE            | 54.42 $\pm$ 0.06 | 55.01 $\pm$ 0.10        | <b>55.70</b> $\pm$ 0.13 | 55.41 $\pm$ 0.15        | 55.03 $\pm$ 0.09        | 54.65 $\pm$ 0.10 | 54.44 $\pm$ 0.13        | 10.00 $\pm$ 0.00 | 10.00 $\pm$ 0.00 |
| MAE           | 49.44 $\pm$ 1.11 | <b>49.86</b> $\pm$ 1.13 | 49.18 $\pm$ 1.82        | 43.03 $\pm$ 1.26        | 22.80 $\pm$ 2.81        | 11.37 $\pm$ 0.97 | 10.92 $\pm$ 0.92        | 10.00 $\pm$ 0.00 | 10.00 $\pm$ 0.00 |
| MAE*          | 52.98 $\pm$ 0.13 | 53.84 $\pm$ 0.05        | 54.20 $\pm$ 0.09        | <b>55.09</b> $\pm$ 0.14 | 42.67 $\pm$ 3.46        | 10.35 $\pm$ 0.35 | 12.20 $\pm$ 0.97        | 10.00 $\pm$ 0.00 | 10.00 $\pm$ 0.00 |
| boundCE       | 51.23 $\pm$ 0.29 | 52.25 $\pm$ 0.17        | 52.61 $\pm$ 0.14        | 54.13 $\pm$ 0.28        | <b>54.38</b> $\pm$ 0.18 | 40.85 $\pm$ 0.31 | 20.60 $\pm$ 3.24        | 10.00 $\pm$ 0.00 | 10.00 $\pm$ 0.00 |
| genCE         | 52.54 $\pm$ 0.16 | 53.54 $\pm$ 0.16        | 53.91 $\pm$ 0.07        | 54.99 $\pm$ 0.18        | <b>55.21</b> $\pm$ 0.13 | 55.02 $\pm$ 0.26 | 54.57 $\pm$ 0.07        | 10.00 $\pm$ 0.00 | 10.00 $\pm$ 0.00 |
| symCE         | 53.63 $\pm$ 0.07 | 54.00 $\pm$ 0.30        | <b>54.13</b> $\pm$ 0.14 | 53.79 $\pm$ 0.11        | 53.61 $\pm$ 0.11        | 52.13 $\pm$ 0.17 | 51.34 $\pm$ 0.23        | 19.22 $\pm$ 6.12 | 10.00 $\pm$ 0.00 |
| actPas1       | 53.67 $\pm$ 0.15 | 53.88 $\pm$ 0.10        | <b>53.98</b> $\pm$ 0.13 | 16.48 $\pm$ 2.93        | 14.92 $\pm$ 1.88        | 10.00 $\pm$ 0.00 | 10.83 $\pm$ 0.83        | 10.46 $\pm$ 0.46 | 10.00 $\pm$ 0.00 |
| actPas2       | 53.82 $\pm$ 0.04 | <b>53.77</b> $\pm$ 0.10 | 53.49 $\pm$ 0.21        | 16.61 $\pm$ 0.81        | 14.12 $\pm$ 1.10        | 13.09 $\pm$ 1.04 | 11.43 $\pm$ 1.43        | 10.00 $\pm$ 0.00 | 10.00 $\pm$ 0.00 |
| biTemp        | 53.17 $\pm$ 0.15 | 54.23 $\pm$ 0.07        | 54.69 $\pm$ 0.18        | 55.89 $\pm$ 0.22        | <b>56.02</b> $\pm$ 0.24 | 55.21 $\pm$ 0.17 | 54.97 $\pm$ 0.18        | 50.76 $\pm$ 0.25 | 28.66 $\pm$ 8.11 |
| Fashion-MNIST |                  |                         |                         |                         |                         |                  |                         |                  |                  |
| CE            | 89.39 $\pm$ 0.06 | 89.63 $\pm$ 0.08        | 89.64 $\pm$ 0.08        | 90.11 $\pm$ 0.05        | <b>90.20</b> $\pm$ 0.03 | 89.97 $\pm$ 0.05 | 90.08 $\pm$ 0.06        | 89.19 $\pm$ 0.10 | 10.00 $\pm$ 0.00 |
| MAE           | 81.24 $\pm$ 2.24 | <b>84.83</b> $\pm$ 2.32 | 82.53 $\pm$ 2.60        | 82.11 $\pm$ 2.21        | 84.34 $\pm$ 2.00        | 79.61 $\pm$ 2.65 | 72.00 $\pm$ 1.88        | 10.03 $\pm$ 0.03 | 12.00 $\pm$ 1.79 |
| MAE*          | 88.72 $\pm$ 0.05 | 88.52 $\pm$ 0.95        | 88.52 $\pm$ 0.95        | <b>89.55</b> $\pm$ 0.03 | 88.52 $\pm$ 0.95        | 89.43 $\pm$ 0.06 | 87.55 $\pm$ 0.52        | 10.00 $\pm$ 0.00 | 10.01 $\pm$ 0.01 |
| boundCE       | 86.81 $\pm$ 0.84 | 87.24 $\pm$ 0.89        | 87.40 $\pm$ 0.90        | 89.11 $\pm$ 0.05        | <b>89.48</b> $\pm$ 0.04 | 89.41 $\pm$ 0.04 | 89.26 $\pm$ 0.06        | 16.68 $\pm$ 4.28 | 10.07 $\pm$ 0.06 |
| genCE         | 88.54 $\pm$ 0.05 | 88.82 $\pm$ 0.03        | 88.93 $\pm$ 0.04        | 89.57 $\pm$ 0.05        | 89.60 $\pm$ 0.08        | 89.75 $\pm$ 0.06 | <b>89.76</b> $\pm$ 0.06 | 17.00 $\pm$ 1.60 | 11.06 $\pm$ 0.95 |
| symCE         | 89.54 $\pm$ 0.06 | 89.84 $\pm$ 0.05        | 89.80 $\pm$ 0.10        | 89.97 $\pm$ 0.09        | <b>89.98</b> $\pm$ 0.07 | 89.68 $\pm$ 0.07 | 89.66 $\pm$ 0.10        | 88.55 $\pm$ 0.04 | 10.00 $\pm$ 0.00 |
| actPas1       | 88.73 $\pm$ 0.05 | 89.06 $\pm$ 0.04        | <b>89.13</b> $\pm$ 0.03 | 88.30 $\pm$ 0.03        | 30.28 $\pm$ 4.61        | 20.34 $\pm$ 7.53 | 17.47 $\pm$ 1.70        | 10.00 $\pm$ 0.00 | 12.36 $\pm$ 1.57 |
| actPas2       | 88.82 $\pm$ 0.03 | 89.05 $\pm$ 0.03        | <b>89.14</b> $\pm$ 0.03 | 88.31 $\pm$ 0.05        | 43.06 $\pm$ 8.93        | 10.00 $\pm$ 0.00 | 13.94 $\pm$ 2.16        | 15.95 $\pm$ 2.17 | 11.87 $\pm$ 1.66 |
| biTemp        | 89.08 $\pm$ 0.03 | 89.33 $\pm$ 0.10        | 89.50 $\pm$ 0.06        | 89.97 $\pm$ 0.06        | 90.13 $\pm$ 0.06        | 90.16 $\pm$ 0.07 | <b>90.19</b> $\pm$ 0.07 | 89.93 $\pm$ 0.06 | 89.44 $\pm$ 0.09 |

### 3 Backpropagation error for bounded losses

For completeness, we provide the backpropagation errors  $\delta_n$  for the active passive and the boundCE losses in this section. As in the main text,  $k$  denotes the index of non-zero entry in the corresponding one-hot encoded label, i.e.  $k = \text{argmax}(\mathbf{y})$ .

The active passive losses are defined as

$$\text{ActPas1} = \alpha \frac{\log((1 - a_k)^{0.5} a_k)}{\sum_i \log((1 - a_i)^{0.5} a_i)} + \beta \text{MAE}(\mathbf{a}, \mathbf{y}), \quad (1)$$

$$\text{ActPas2} = \alpha \frac{\log(a_k)}{\sum_i \log(a_i)} + \beta \text{MAE}(\mathbf{a}, \mathbf{y}). \quad (2)$$

We are interested in the error  $\delta_n = \partial_{z_n} \mathcal{L}$  where  $a_i = \exp(z_n) / \sum_i \exp z_i$ . The derivative of the mean absolute error (MAE) is given in the Manuscript as  $2a_k(a_k - \delta_{nk})$ . We further find that

$$\begin{aligned} \frac{\partial}{\partial z_n} \frac{\log((1 - a_k)^{0.5} a_k)}{\sum_i \log((1 - a_i)^{0.5} a_i)} &= \\ \frac{(\delta_{nk} - a_n) \left(1 - \frac{a_k}{2 - 2a_k}\right) \left(\sum_i \log((1 - a_i)^{0.5} a_i)\right) - \left(\sum_i (\delta_{ni} - a_n) \left(1 - \frac{a_i}{2 - 2a_i}\right) \log((1 - a_k)^{0.5} a_k)\right)}{\left(\sum_i \log((1 - a_i)^{0.5} a_i)\right)^2}, \\ \frac{\partial}{\partial z_n} \frac{\log(a_k)}{\sum_i \log(a_i)} &= \frac{(\delta_{nk} - a_n) \sum_i \log(a_i) - \log(a_k)(-ca_n + 1)}{\left(\sum_i \log(a_i)\right)^2}. \end{aligned} \quad (3)$$

A visualization of these formulas is provided by the *learning curves* in the main manuscript.

For the Bounded Cross Entropy

$$\text{boundCE}(z, y) = -\ln \left( \frac{\exp a_k}{\sum_i^c \exp(a_i)} \right), \quad a_i = \frac{\exp z_i}{\sum_j^c \exp(z_j)} \quad (4)$$

we find the error

$$\frac{\partial \text{boundCE}}{\partial z_n} = -a_k (\delta_{nk} - a_n) + \frac{a_n}{\sum_j \exp(a_j)} \left( \exp(a_n) - \sum_j a_j \exp(a_j) \right). \quad (5)$$
